# Supplementary material for: PolyOCR-Venus: Unified OCR Foundation Models for Text-Centric Visual Intelligence
Source: arXiv:2609.37712 source file (2026-09-29)
Supplement: Supplementary file 1 [file 8_appendix.tex]

\section{Training Data Composition}
\label{app:data_composition}

Table~\ref{tab:training_data_composition} summarizes the domain-wise composition of the 12.5M training samples used for DeFakerOne. The training data covers four FIDL domains, including DeepFake, AIGC, Document, and Nature. For each domain, we combine public datasets with private real-world data when available, and apply domain-specific sampling to avoid over-dominance from any single dataset.
\input{tab/tab_dataset_consist}



\section{Contributors}
\label{sec:contri}

\large{All contributors are listed \textbf{alphabetically by the first name}.} 

\large{
\begin{minipage}[t]{0.48\textwidth} % 左侧栏
    \textbf{Core Contributors} \\
    XXX
    \vspace{0.4cm} \\
    \textbf{Contributors} \\
    Chenfeng Zhang \\
    Longfei Liu
\end{minipage}
\hfill
\begin{minipage}[t]{0.48\textwidth} % 右侧栏
    \textbf{Data Leader} \\
    Zhenming Wang \\
    \vspace{0.4cm} \\
    \textbf{Project Leader} \\
    Jian Liu \\
    Jingjing Liu \\
    \vspace{0.4cm} \\
    \textbf{Project Advisor} \\
    Weiqiang Wang
\end{minipage}
}

\input{tab/tab_robust_full}

%\section{Open-source image data}
%\label{sec:app_image_data}
%In addition to the open source image data utilized in \citep{guo2025m2}, the newly added data are presented in Table~\ref{tab:image_data}.


%\section{Open-source audio data}
%\label{sec:app_audio_data}
%We include the complete list of open source audio data we used during our training in Table~\ref{tab:audio_data}.


%\section{Open-source video data}
%\label{sec:app_video_data}

%The comprehensive list of open-source video datasets utilized during the training process is provided in Table~\ref{tab:vieo_data}.
